# Supplementary material for: DKWS: A Distributed System for Keyword Search on Massive Graphs (Complete Version)
Source: arXiv:2309.01199 source file (2023-09-09)
Supplement: Supplementary file 1 [file exp-query-performance-appendix.tex]

\begin{figure*}[tp]
	%\vspace{-0.2cm}
		\begin{minipage}{\linewidth}
	
		\begin{tabular}{cc}
		% 1.1
		\begin{minipage}[t]{0.24\textwidth} 
		\includegraphics[width=\textwidth]{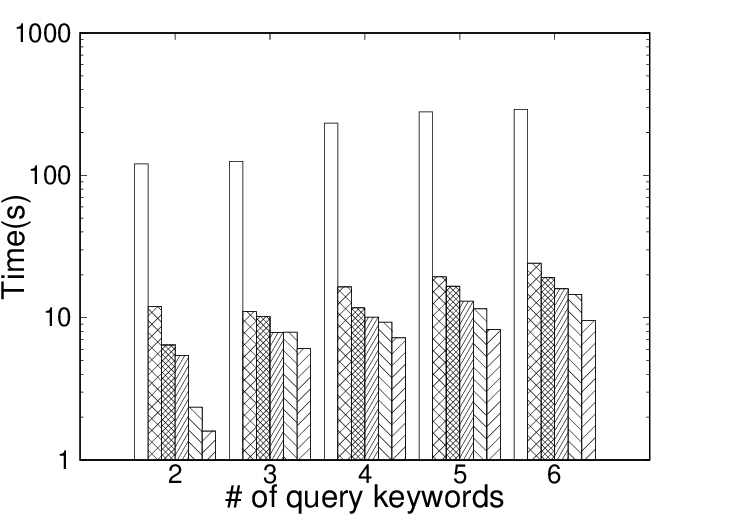}
		\subcaption{\footnotesize Vary $\#$ of query keywords (YAGO3)}
		\label{fig:dkws-baseline-yago-appdix}
		\end{minipage}
		% 1.4
		\begin{minipage}[t]{0.24\textwidth} 
			\includegraphics[width=\textwidth]{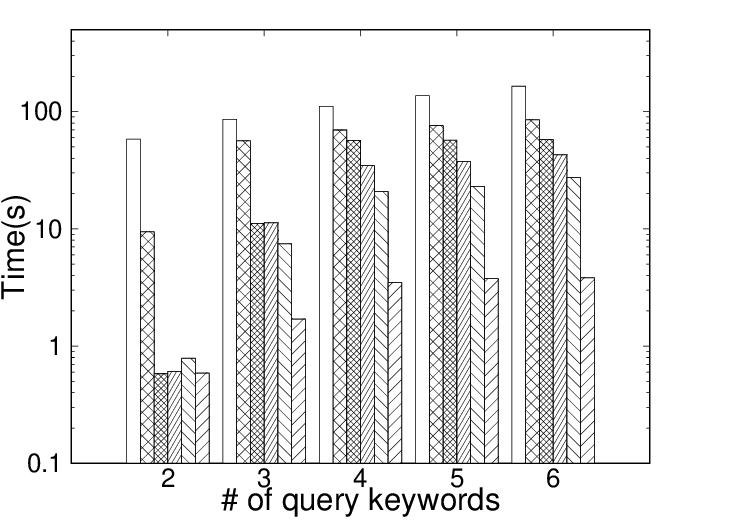}
			\subcaption{\footnotesize Vary $\#$ of query keywords  (DBpedia)}			\label{fig:dkws-baseline-dbpedia-appdix}
			\end{minipage}
		\end{tabular}

%%%%%%%% Followings are messages. For backup. 
\eat{
		\begin{tabular}{cc}
			% 3.1
		\begin{minipage}[t]{0.24\textwidth} 
			\includegraphics[width=\textwidth]{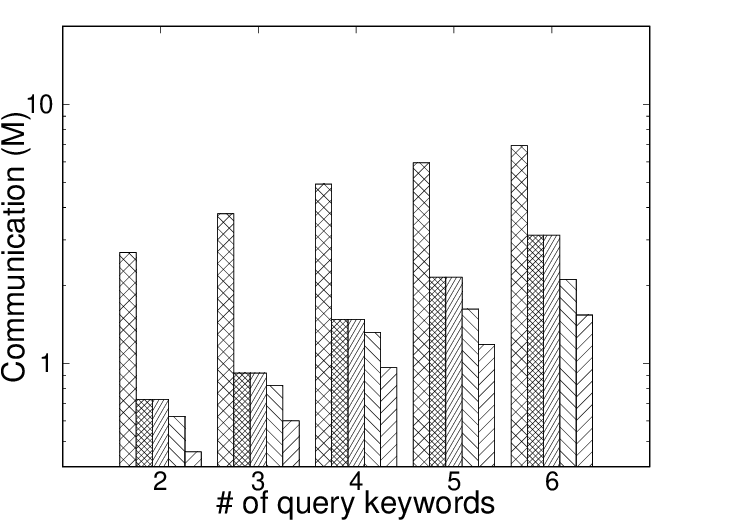}
			\subcaption{Vary $\#$ of query keywords (YAGO3)}
			\label{fig:dkws-baseline-msg-yago}
		\end{minipage}
		% 3.2
		\begin{minipage}[t]{0.24\textwidth} 
			\includegraphics[width=\textwidth]{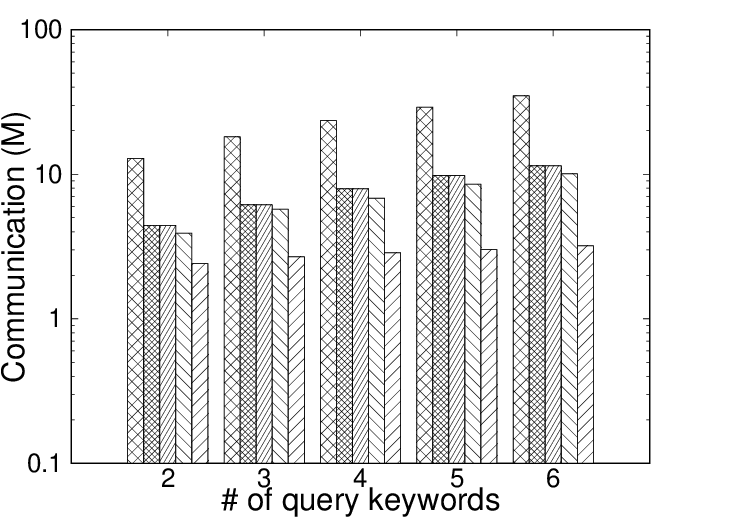}
			\subcaption{Vary $\#$ of query keywords (WebUK)}
			\label{fig:dkws-baseline-msg-webuk}
		\end{minipage}
		% 3.3
		\begin{minipage}[t]{0.24\textwidth} 
			\includegraphics[width=\textwidth]{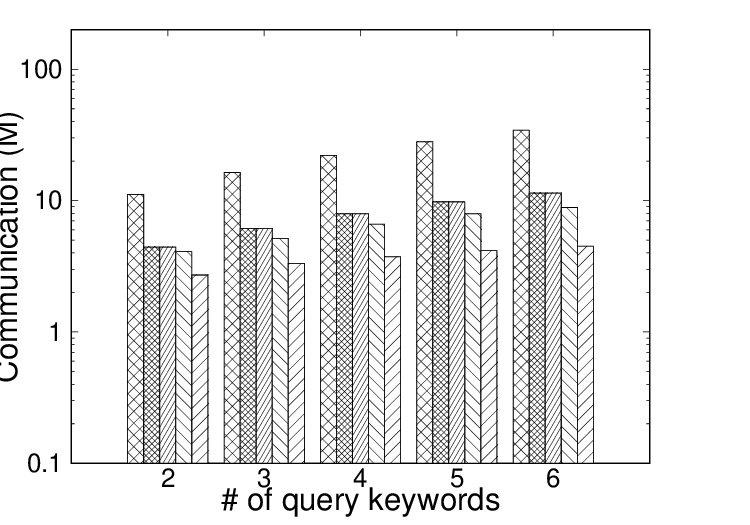}
			\subcaption{Vary $\#$ of query keywords (DBLP)}
			\label{fig:dkws-baseline-msg-dblp}
		\end{minipage}
			% 3.4
		\begin{minipage}[t]{0.24\textwidth} 
			\includegraphics[width=\textwidth]{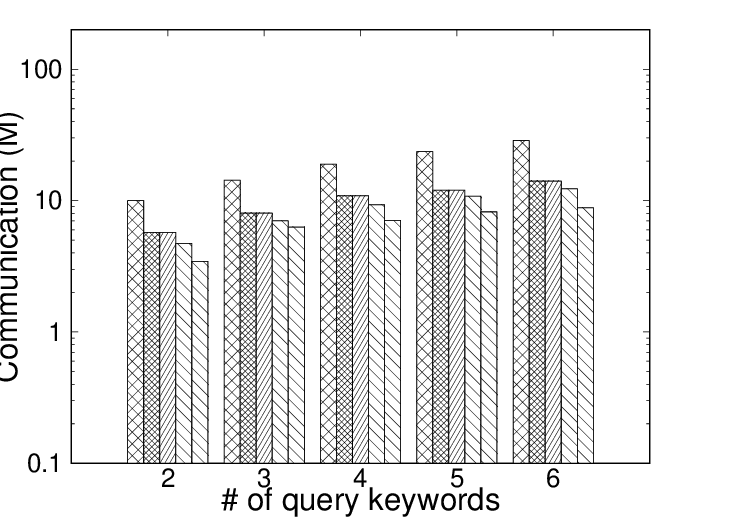}
			\subcaption{Vary $\#$ of query keywords (DBpedia)}
			\label{fig:dkws-baseline-msg-dbpedia}
		\end{minipage}
		\end{tabular}
		
		\begin{tabular}{cc}
			% 4.1 
			\begin{minipage}[t]{0.24\textwidth} 
				\includegraphics[width=\textwidth]{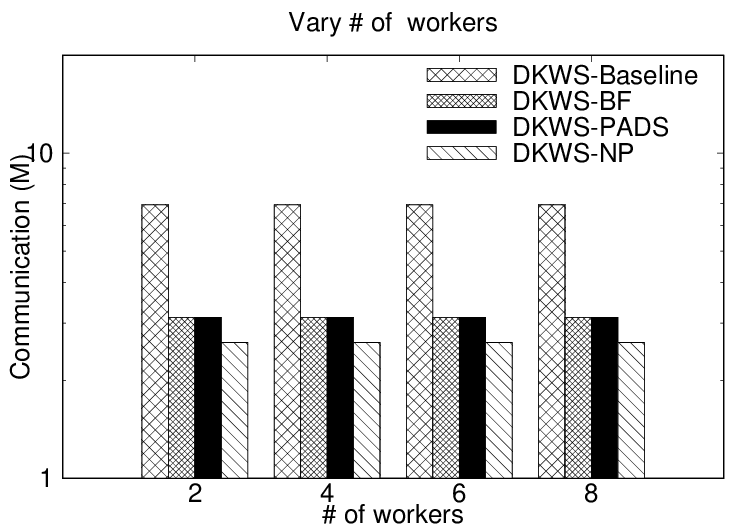}
				\subcaption{\footnotesize Vary $\#$ of the workers (YAGO3)}
				\label{fig:dkws-vary-workers-msg-yago}
			\end{minipage}
				  % 4.2
			\begin{minipage}[t]{0.24\textwidth} 
				\includegraphics[width=\textwidth]{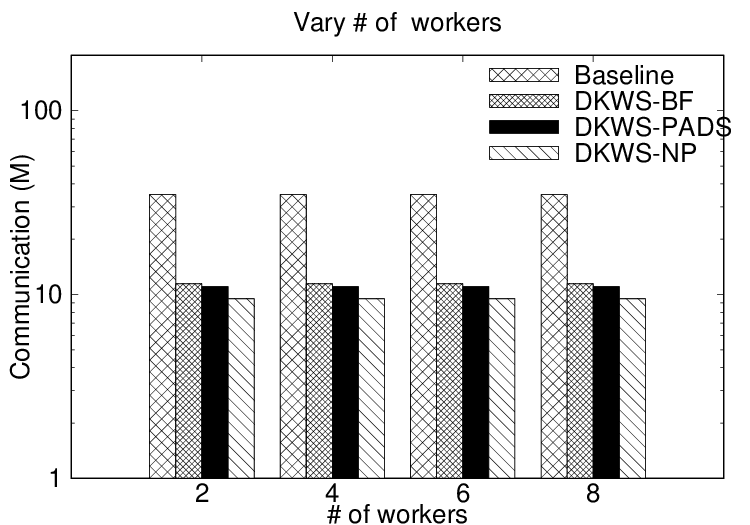}
				\subcaption{\footnotesize Vary $\#$ of the workers (WebUK)}
				\label{fig:dkws-vary-workers-msg-webuk}
			\end{minipage}
				  % 4.3
				  \begin{minipage}[t]{0.24\textwidth} 
					\includegraphics[width=\textwidth]{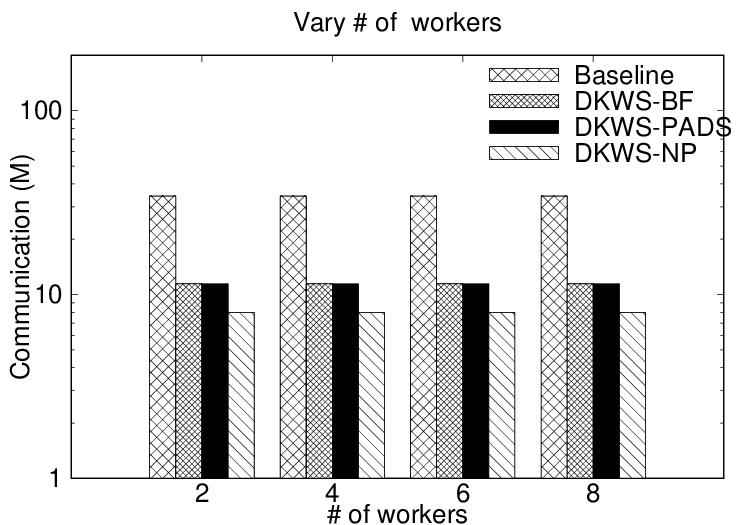}
					\subcaption{\footnotesize Vary $\#$ of the workers (DBLP)}
					\label{fig:dkws-vary-workers-msg-webuk}
				\end{minipage}
				% 4.4
				\begin{minipage}[t]{0.24\textwidth} 
					\includegraphics[width=\textwidth]{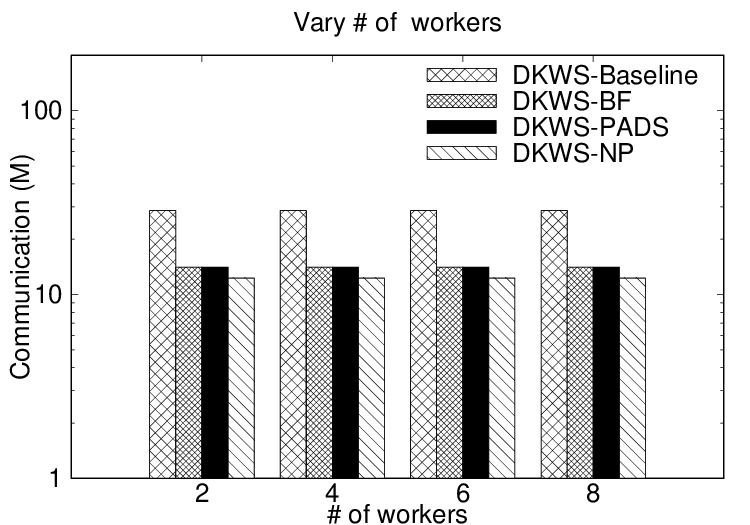}
					\subcaption{\footnotesize Vary $\#$ of the workers (DBpedia)}
					\label{fig:dkws-vary-workers-msg-dbpedia}
				\end{minipage}
		\end{tabular}
}		
	\caption{Performance on the two extra datasets}
	\label{fig:performance-appendix}
		\end{minipage}
	%        \vspace{-1cm}
	\end{figure*}
